# Supplementary material for: Bias in Internet Measurement Platforms
Source: arXiv:2307.09958 source file (2023-07-24)
Supplement: Supplementary file 1 [file appendix_short.tex]

\section{Distributions of the Infrastructure Characteristics}\label{appendix:distributions}
Figures~\ref{fig:appendix-distribution-characteristics1} %, ~\ref{fig:appendix-distribution-characteristics2}, 
and~\ref{fig:appendix-distribution-characteristics3} present the detailed distributions of the characteristics we consider (see~\secref{sec:bias-dimensions}) for the entire population of ASes and for the ASes in the \imps.

\begin{figure}
\centering
    \subfigure[RIR region]{\includegraphics[width=0.3\linewidth]{./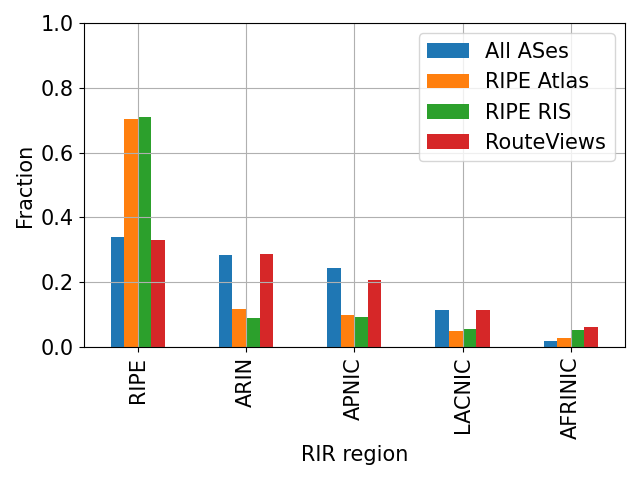}}
    \hspace{0.2\linewidth}
    \subfigure[Location (continent)]{\includegraphics[width=0.32\linewidth]{./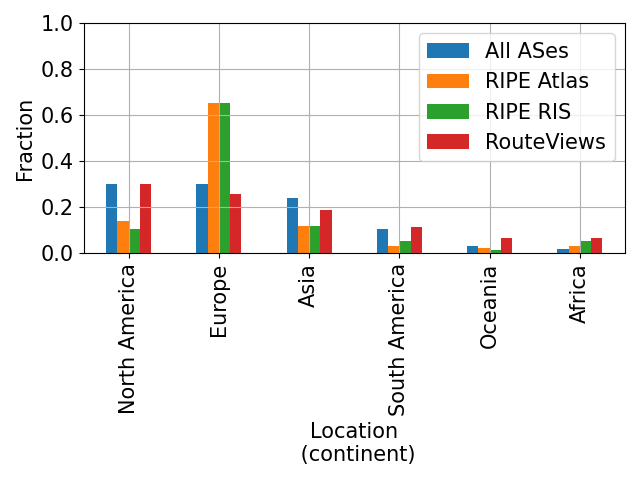}}
    \caption{Location dimensions}
    \label{fig:appendix-distribution-characteristics1}
\end{figure}

\begin{figure}
\centering
    \textbf{Network size dimensions}\\
    \subfigure[Customer cone (\#ASNs)]{\includegraphics[width=0.24\linewidth]{./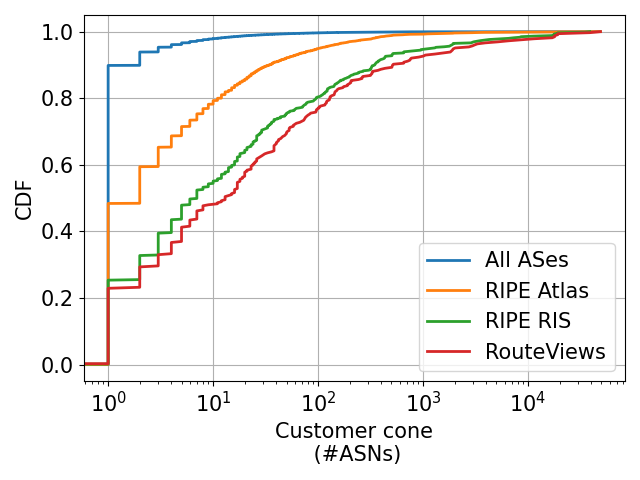}}
    \subfigure[Customer cone (\#prefixes)]{\includegraphics[width=0.24\linewidth]{./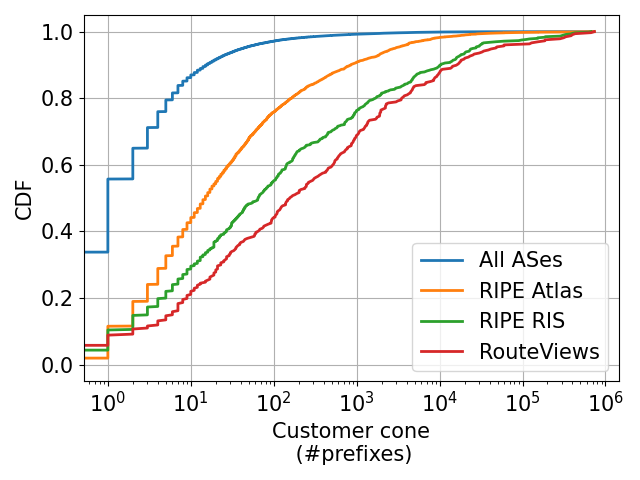}}
    \subfigure[Customer cone (\#addresses)]{\includegraphics[width=0.24\linewidth]{./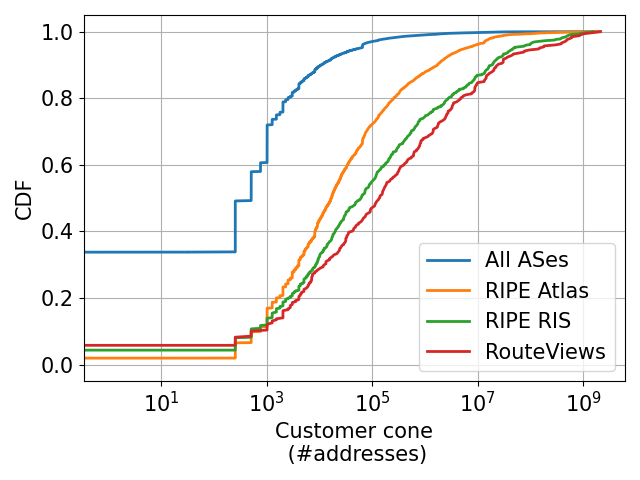}}
    \subfigure[AS hegemony]{\includegraphics[width=0.24\linewidth]{./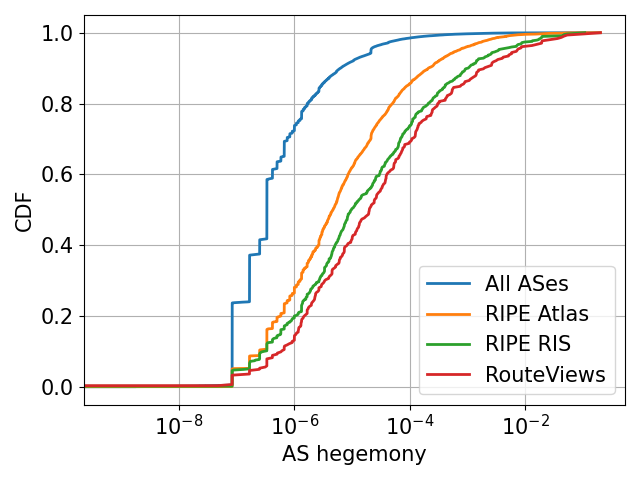}}\\
    \textbf{Topology dimensions}\\
    \subfigure[\#neighbors (total)]{\includegraphics[width=0.24\linewidth]{./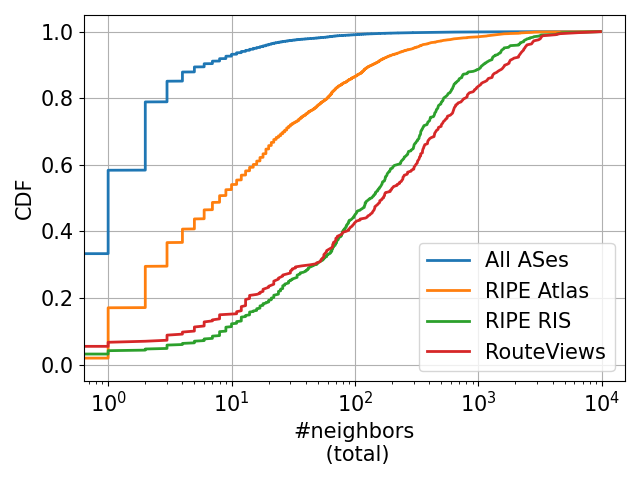}}
    \subfigure[\#neighbors (peers)]{\includegraphics[width=0.24\linewidth]{./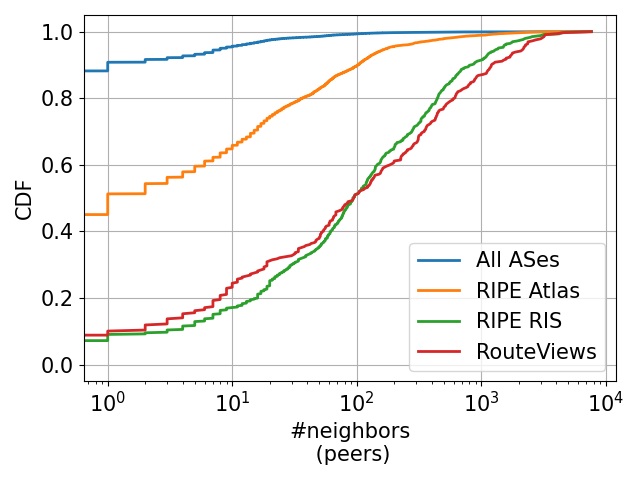}}
    \subfigure[\#neighbors (customers)]{\includegraphics[width=0.24\linewidth]{./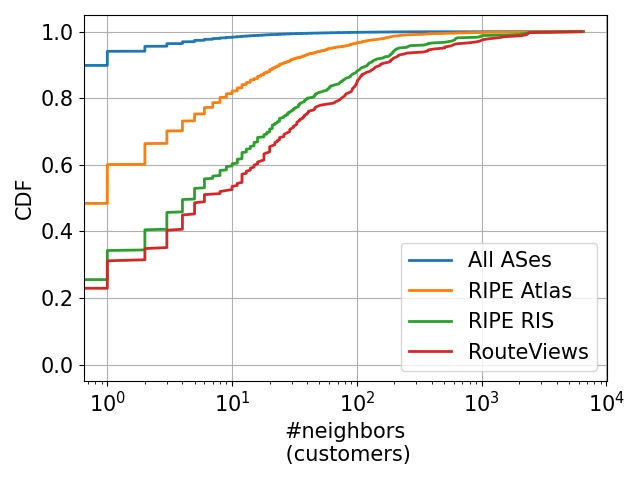}}
    \subfigure[\#neighbors (providers)]{\includegraphics[width=0.24\linewidth]{./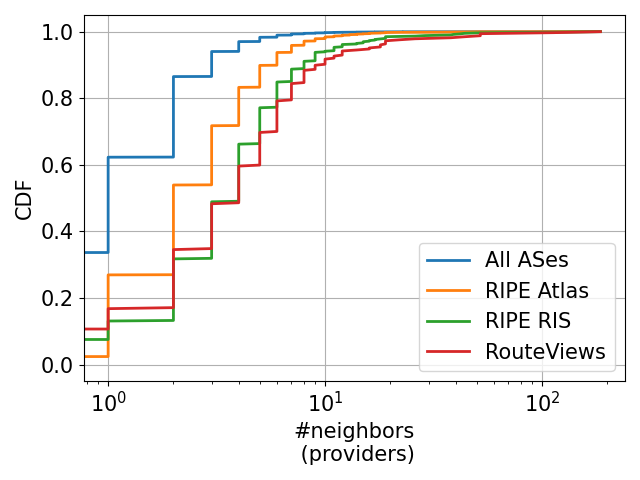}}
    % \caption{Network size and Topology dimensions}
    % \label{fig:appendix-distribution-characteristics2}
% \end{figure}

% \begin{figure}
% \centering
    \textbf{Interconnection (IXP-related) dimensions}\\
    \subfigure[\#IXPs]{\includegraphics[width=0.24\linewidth]{./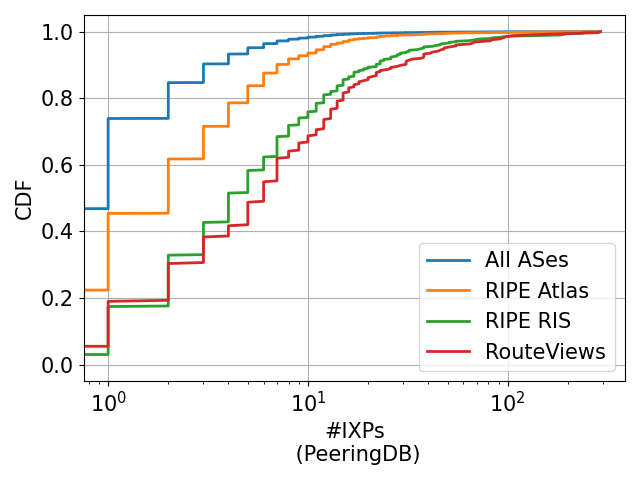}}
    \subfigure[\#facilities]{\includegraphics[width=0.24\linewidth]{./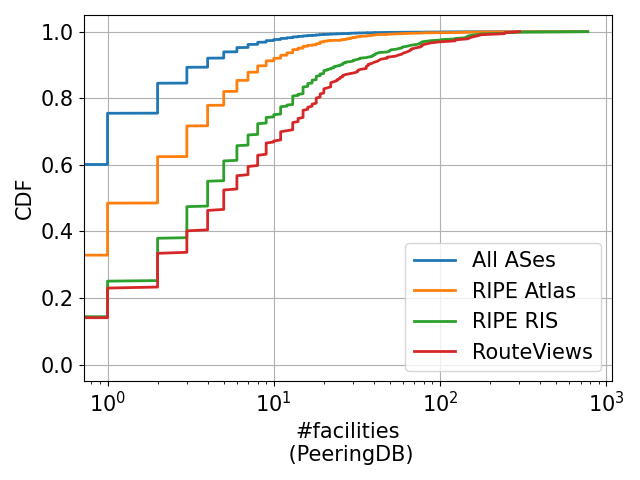}}
    \subfigure[Peering policy]{\includegraphics[width=0.24\linewidth]{./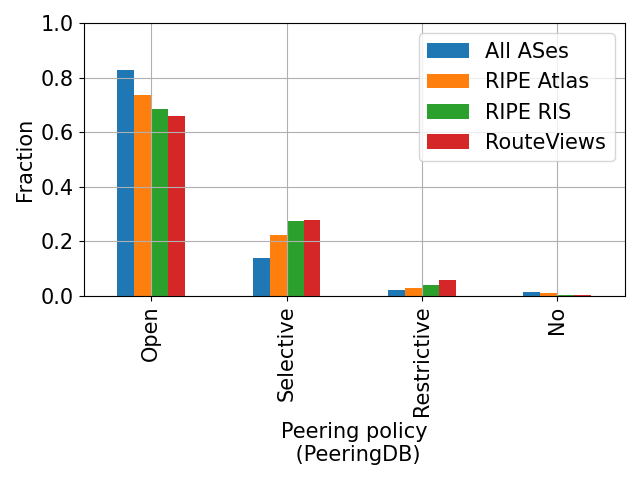}}\\
    \textbf{Network type dimensions}\\
    \subfigure[Network type]{\includegraphics[width=0.24\linewidth]{./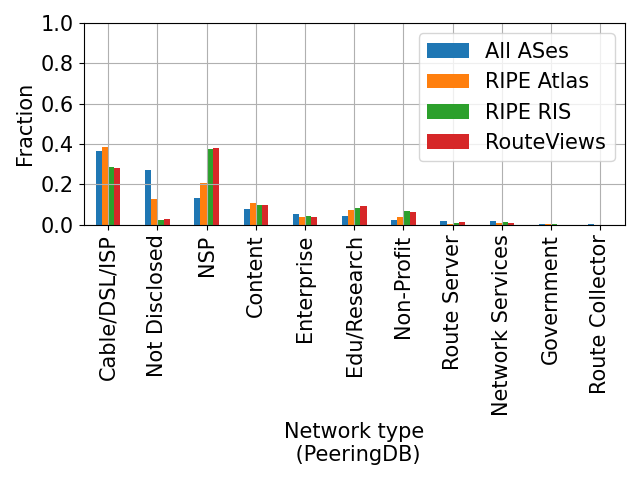}}
    \subfigure[Traffic ratio]{\includegraphics[width=0.24\linewidth]{./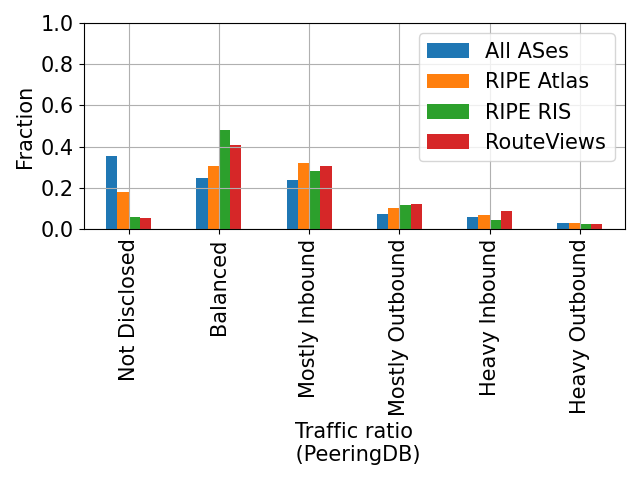}}
    \subfigure[Traffic volume]{\includegraphics[width=0.24\linewidth]{./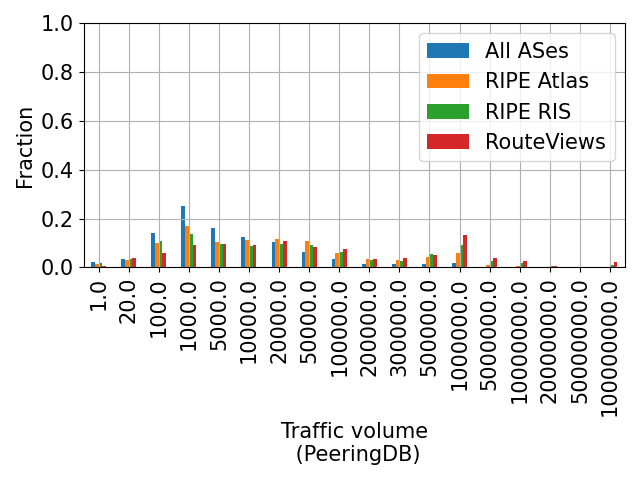}}
    \subfigure[Scope]{\includegraphics[width=0.24\linewidth]{./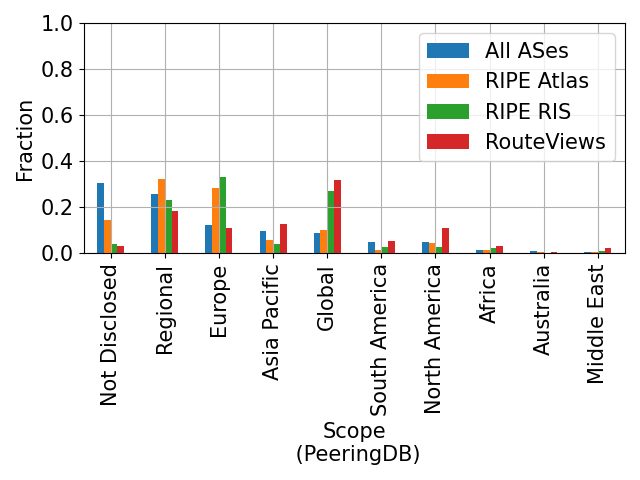}}
    % \subfigure[Personal ASN]{\includegraphics[width=0.24\linewidth]{./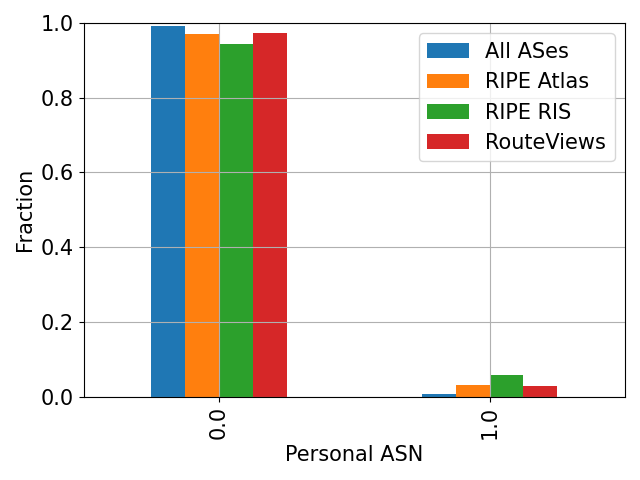}}
    \caption{Network size, Topology, Interconnection (IXP-related) and Network type dimensions.}
    \label{fig:appendix-distribution-characteristics3}
\end{figure}
