# Supplementary material for: Bias in Internet Measurement Platforms
Source: arXiv:2307.09958 source file (2023-07-24)
Supplement: Supplementary file 2 [file appendix_distributions.tex]

Figure%s~\ref{fig:appendix-distribution-characteristics1} and
~\ref{fig:appendix-distribution-characteristics2} presents the detailed distributions of the characteristics we consider (see~\secref{sec:bias-dimensions}) for the entire population of ASes and for the ASes in the \imps.

\begin{figure}
\centering
    \textbf{Location \& Network size dimensions}\\
    \subfigure[RIR region]{\includegraphics[width=0.24\linewidth]{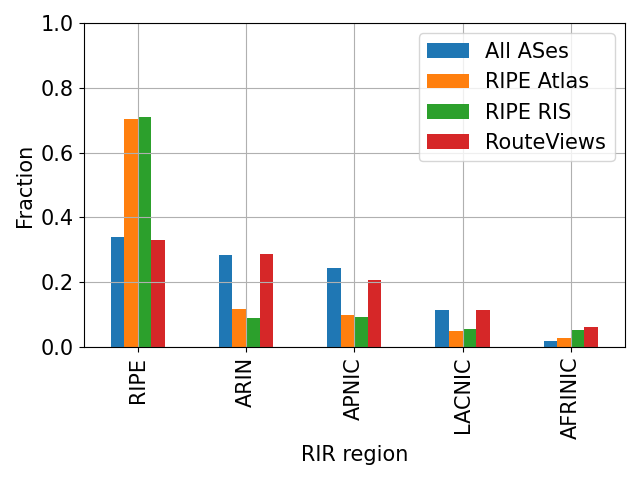}}
    \subfigure[Location (continent)]{\includegraphics[width=0.24\linewidth]{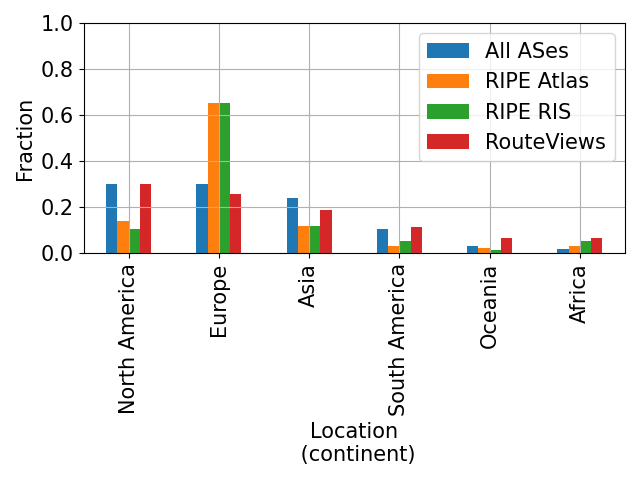}}%\\
    % \textbf{Network size dimensions}\\
    \subfigure[Customer cone (\#ASNs)]{\includegraphics[width=0.24\linewidth]{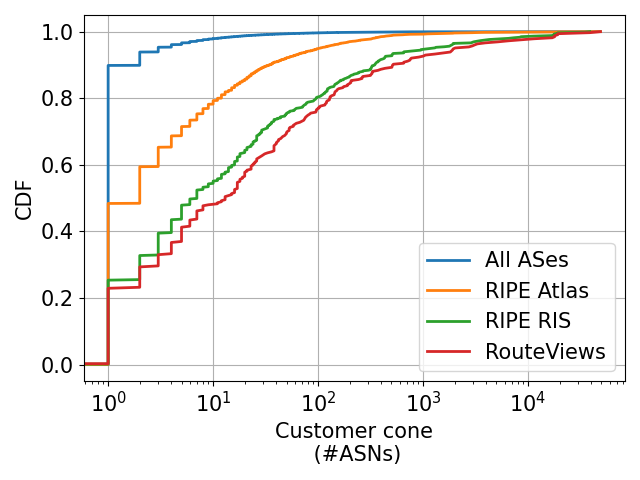}}
    % \subfigure[Customer cone (\#prefixes)]{\includegraphics[width=0.24\linewidth]{./figures/distributions/Fig_CDF_AS_rank_numberPrefixes.png}}
    % \subfigure[Customer cone (\#addresses)]{\includegraphics[width=0.24\linewidth]{./figures/distributions/Fig_CDF_AS_rank_numberAddresses.png}}
    \subfigure[AS hegemony]{\includegraphics[width=0.24\linewidth]{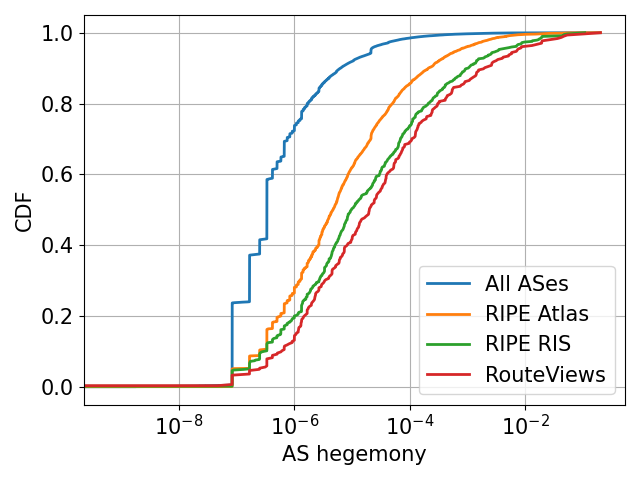}}\\
    \textbf{Topology dimensions}\\
    \subfigure[\#neighbors (total)]{\includegraphics[width=0.24\linewidth]{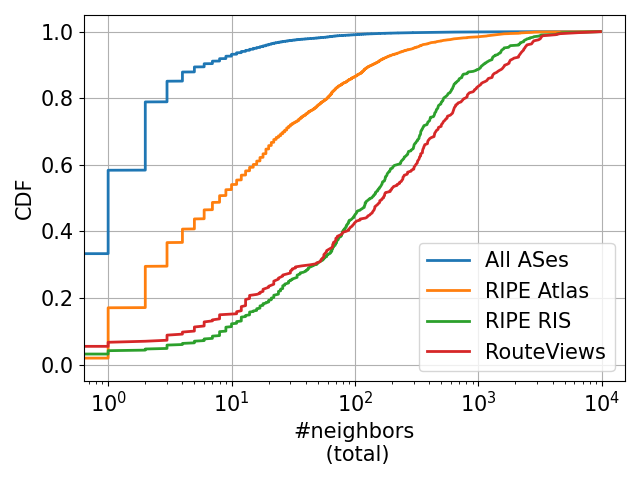}}
    \subfigure[\#neighbors (peers)]{\includegraphics[width=0.24\linewidth]{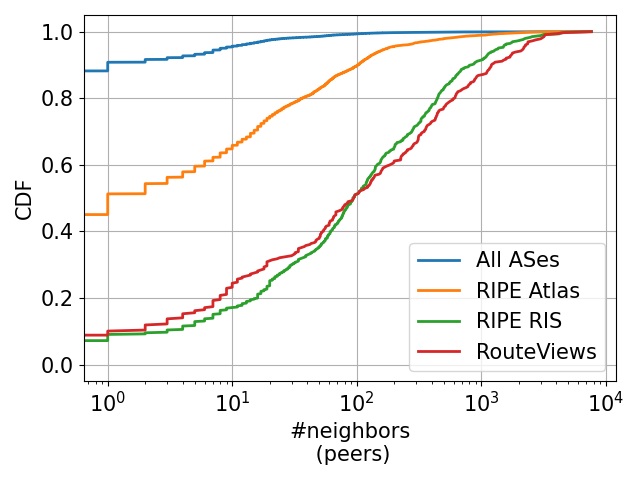}}
    \subfigure[\#neighbors (customers)]{\includegraphics[width=0.24\linewidth]{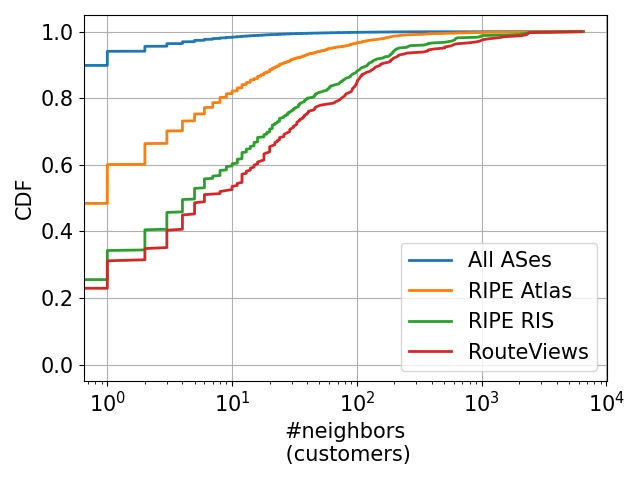}}
    \subfigure[\#neighbors (providers)]{\includegraphics[width=0.24\linewidth]{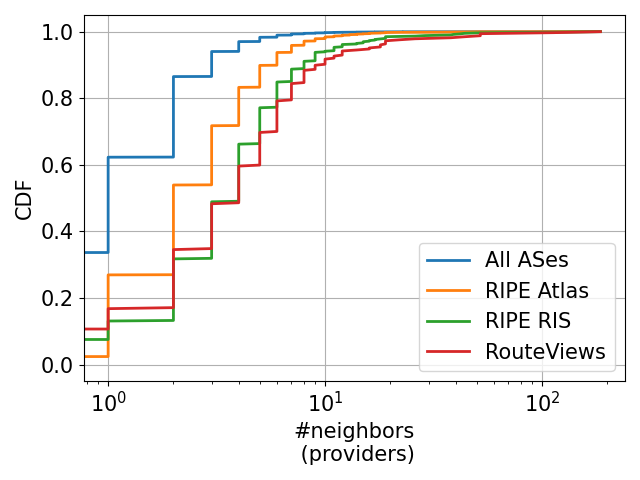}}%
    \\
    \textbf{Interconnection (IXP-related) dimensions}\\
    \subfigure[\#IXPs]{\includegraphics[width=0.24\linewidth]{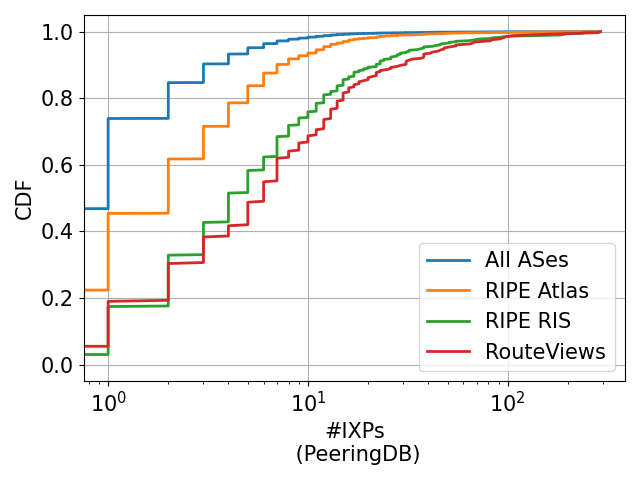}}
    \subfigure[\#facilities]{\includegraphics[width=0.24\linewidth]{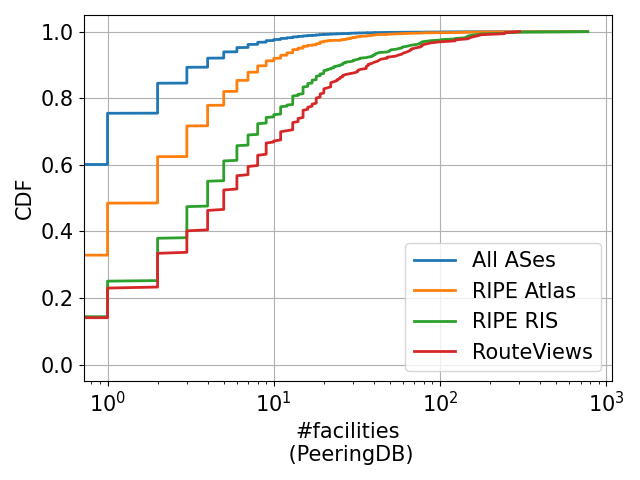}}
    \subfigure[Peering policy]{\includegraphics[width=0.24\linewidth]{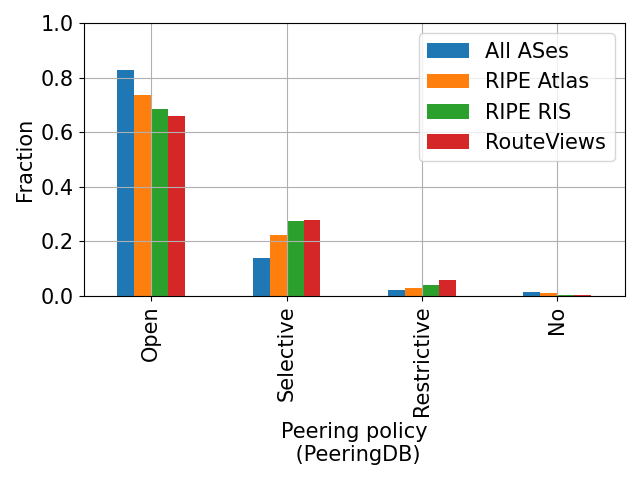}}\\
    \textbf{Network type dimensions}\\
    \subfigure[Network type]{\includegraphics[width=0.24\linewidth]{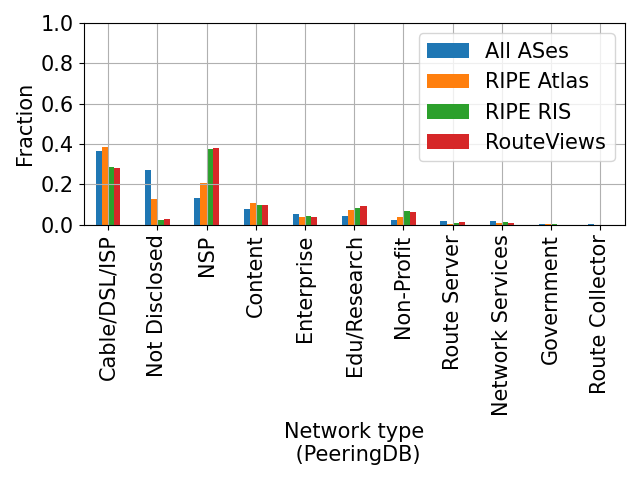}}
    \subfigure[Traffic ratio]{\includegraphics[width=0.24\linewidth]{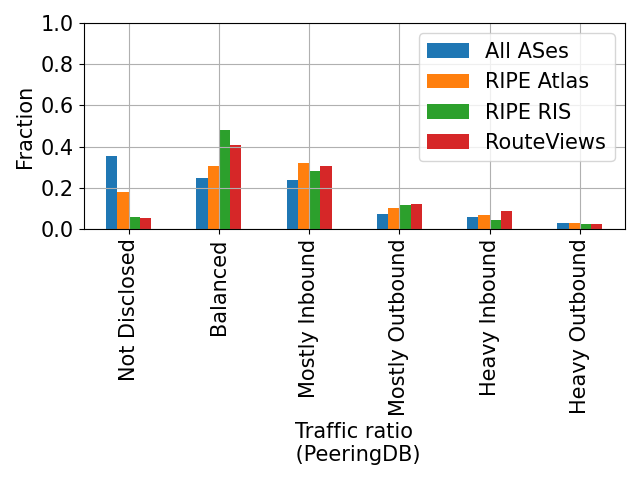}}
    \subfigure[Traffic volume]{\includegraphics[width=0.24\linewidth]{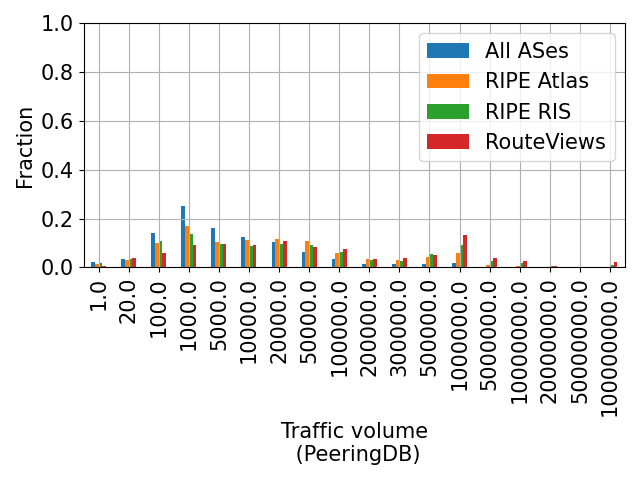}}
    \subfigure[Scope]{\includegraphics[width=0.24\linewidth]{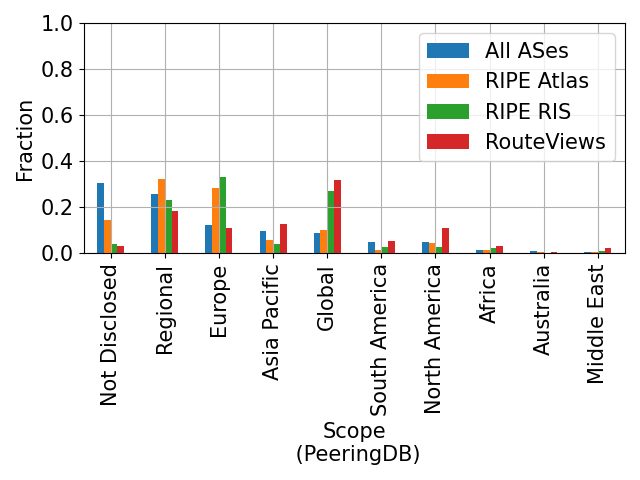}}
    % \subfigure[Personal ASN]{\includegraphics[width=0.24\linewidth]{./figures/distributions/Fig_Histogram_is_personal_AS.png}}
    \caption{Distributions of different characteristics for the entire population of ASes and the set of ASes that are part of the \imps.}
    \label{fig:appendix-distribution-characteristics2}
\end{figure}
